# Supplementary material for: AIC CTU system at AVeriTeC: Re-framing automated fact-checking as a simple RAG task
Source: arXiv:2410.11446 source file (2024-10-15)
Supplement: Supplementary file 1 [file appendix_b_opensource.tex]

%!TEX ROOT=../emnlp2023.tex

\section{Open-Source LLMs}
\label{appendix_sec:opensource_llms}
